# Supplementary material for: Enforcing stationarity through the prior in vector autoregressions
Source: arXiv:2004.09455 ancillary file (2022-05-17)
Supplement: Supplementary file 1 [file supplMat.pdf]

# Supporting materials for *Enforcing stationarity through the prior in vector autoregressions* by Sarah E. Heaps

Sarah E. Heaps
Newcastle University, Newcastle upon Tyne, U.K.
Email: sarah.heaps@ncl.ac.uk

## S1 Graphical illustration

Figure S1 corresponds to Figure 2 in the manuscript, but visualises the prior for the off-diagonal, rather than diagonal, elements.

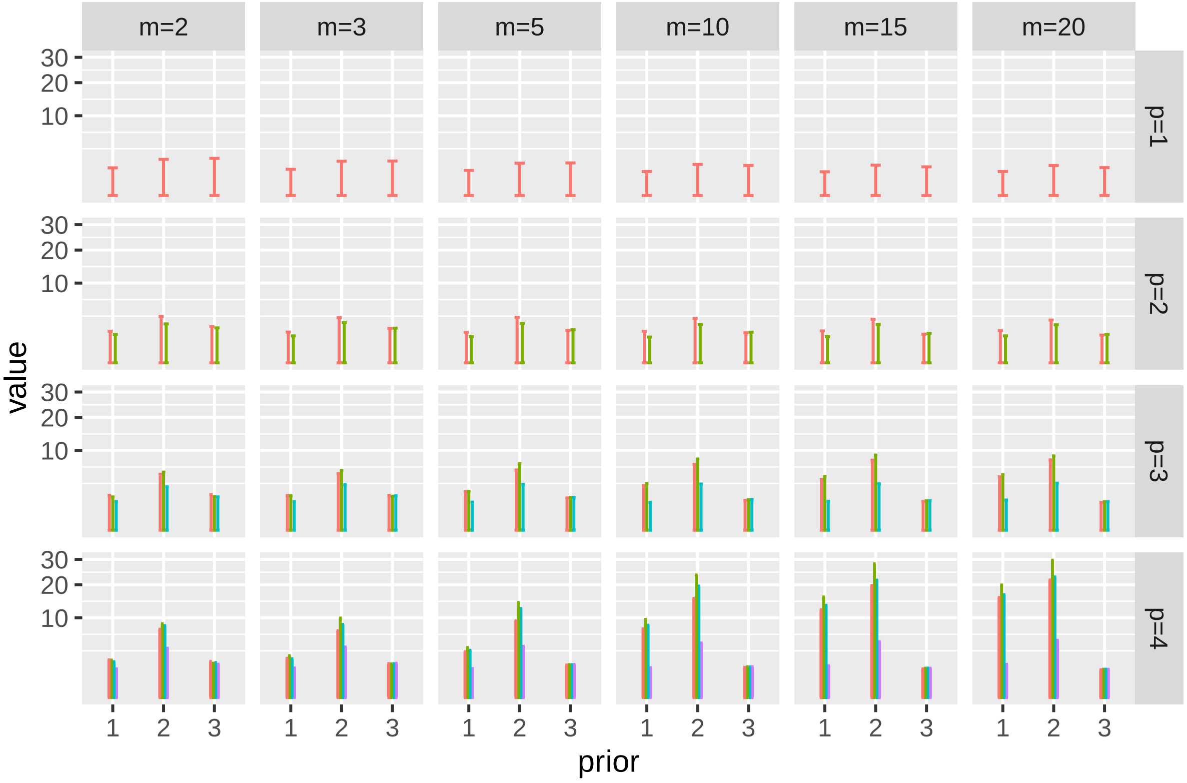


Figure S1: For various choices of $m$ and $p$, panels visualise the upper half of the distribution of the diagonal elements in $\phi_1$ (—) and, where appropriate, $\phi_2$ (—), $\phi_3$ (—) and $\phi_4$ (—) under Priors 1, 2, and 3. The complete distributions are symmetric about zero. Arrows extend from the median to the 95% quantile on a square-root scale.

## S2 Proofs of mappings between the VAR$_m(p)$ parameters and partial autocorrelations

### S2.1 Definitions and preliminary results

For $s = 1, \ldots, p$ let $G_s$ and $g_s$ be $ms \times ms$ and $ms \times m$ block matrices defined as

$$G_s = \begin{pmatrix} \Gamma_0 & \Gamma_1^T & \cdots & \Gamma_{s-1}^T \\ \Gamma_1 & \Gamma_0 & \cdots & \Gamma_{s-2}^T \\ \vdots & \vdots & \ddots & \vdots \\ \Gamma_{s-1} & \Gamma_{s-2} & \cdots & \Gamma_0 \end{pmatrix} \quad \text{and} \quad g_s = \begin{pmatrix} \Gamma_1 \\ \Gamma_2 \\ \vdots \\ \Gamma_s \end{pmatrix}$$

with blockwise transposes denoted by

$$G_s^* = \begin{pmatrix} \Gamma_0 & \Gamma_1 & \cdots & \Gamma_{s-1} \\ \Gamma_1^T & \Gamma_0 & \cdots & \Gamma_{s-2} \\ \vdots & \vdots & \ddots & \vdots \\ \Gamma_{s-1}^T & \Gamma_{s-2}^T & \cdots & \Gamma_0 \end{pmatrix} \quad \text{and} \quad g_s^* = \begin{pmatrix} \Gamma_1^T \\ \Gamma_2^T \\ \vdots \\ \Gamma_s^T \end{pmatrix}.$$

Now denote by $\tilde{g}_s$ and $\tilde{g}_s^*$ the reversed matrices

$$\tilde{g}_s = Q g_s = \begin{pmatrix} \Gamma_s \\ \Gamma_{s-1} \\ \vdots \\ \Gamma_1 \end{pmatrix} \quad \text{and} \quad \tilde{g}_s^* = Q g_s^* = \begin{pmatrix} \Gamma_s^T \\ \Gamma_{s-1}^T \\ \vdots \\ \Gamma_1^T \end{pmatrix}$$

in which the $ms \times ms$ block matrix $Q$, defined by

$$Q = \begin{pmatrix} 0_m & \cdots & 0_m & I_m \\ 0_m & \cdots & I_m & 0_m \\ \vdots & \ddots & \vdots & \vdots \\ I_m & \cdots & 0_m & 0_m \end{pmatrix}$$

is involutory (i.e. its own inverse), symmetric and hence orthogonal.

Let $\boldsymbol{y}_{i:j} = (\boldsymbol{y}_i^T, \ldots, \boldsymbol{y}_j^T)^T$ and

$$\Phi_s = \begin{pmatrix} \phi_{s1}^T \\ \vdots \\ \phi_{ss}^T \end{pmatrix} \quad \text{and} \quad \Phi_{s,-s} = \begin{pmatrix} \phi_{s1}^T \\ \vdots \\ \phi_{s,s-1}^T \end{pmatrix}.$$

Similarly, define

$$\Phi_s^* = \begin{pmatrix} \phi_{s1}^{*T} \\ \vdots \\ \phi_{ss}^{*T} \end{pmatrix} \quad \text{and} \quad \Phi_{s,-s}^* = \begin{pmatrix} \phi_{s1}^{*T} \\ \vdots \\ \phi_{s,s-1}^{*T} \end{pmatrix}.$$

Denote by $\mathbf{0}_m$ the $m$-vector of zeros. Using standard multivariate normal theory, the conditional mean of $\boldsymbol{y}_{t+1}$ given its $s$ predecessors $\boldsymbol{y}_{t:t-s+1}$ is given by

$$\begin{aligned} \mathrm{E}(\boldsymbol{y}_{t+1}|\boldsymbol{y}_{t:t-s+1}) &= \mathrm{E}(\boldsymbol{y}_{t+1}) + \mathrm{Cov}(\boldsymbol{y}_{t+1}, \boldsymbol{y}_{t:t-s+1})\mathrm{Var}(\boldsymbol{y}_{t:t-s+1})^{-1}\{\boldsymbol{y}_{t:t-s+1} - \mathrm{E}(\boldsymbol{y}_{t:t-s+1})\} \\ &= \mathbf{0}_m + g_s^T G_s^{-1}(\boldsymbol{y}_{t:t-s+1} - \mathbf{0}_m) \\ &= g_s^T G_s^{-1}\boldsymbol{y}_{t:t-s+1} \\ &= \Phi_s^T \boldsymbol{y}_{t:t-s+1} \end{aligned}$$

for $s = 1, \ldots, p$, by definition. Therefore

$$\Phi_s = G_s^{-1} g_s \iff g_s = G_s \Phi_s, \quad s = 1, \ldots, p, \tag{S1}$$

in which we refer to the equations on the right as the *forward prediction equations.*

The corresponding conditional variance is given by

$$\begin{aligned}
\operatorname{Var}(\boldsymbol{y}_{t+1}|\boldsymbol{y}_{t:t-s+1}) &= \operatorname{Var}(\boldsymbol{y}_{t+1}) - \operatorname{Cov}(\boldsymbol{y}_{t+1}, \boldsymbol{y}_{t:t-s+1})\operatorname{Var}(\boldsymbol{y}_{t:t-s+1})^{-1}\operatorname{Cov}(\boldsymbol{y}_{t:t-s+1}, \boldsymbol{y}_{t+1}) \\
&= \Gamma_0 - g_s^T G_s^{-1} g_s \\
&= \Gamma_0 - g_s^T \Phi_s \\
&= \Sigma_s
\end{aligned}$$

for $s = 1, \ldots, p$, by definition. By symmetry, this gives

$$\Sigma_s = \Gamma_0 - \Phi_s^T g_s, \quad s = 1, \ldots, p. \tag{S2}$$

Similarly, the conditional mean of $\boldsymbol{y}_{t-s}$ given its $s$ successors $\boldsymbol{y}_{(t-s+1):t}$ is given by

$$\begin{aligned}
\operatorname{E}(\boldsymbol{y}_{t-s}|\boldsymbol{y}_{(t-s+1):t}) &= \operatorname{E}(\boldsymbol{y}_{t-s}) + \operatorname{Cov}(\boldsymbol{y}_{t-s}, \boldsymbol{y}_{(t-s+1):t})\operatorname{Var}(\boldsymbol{y}_{(t-s+1):t})^{-1}\left\{\boldsymbol{y}_{(t-s+1):t} - \operatorname{E}(\boldsymbol{y}_{(t-s+1):t})\right\} \\
&= \mathbf{0}_m + {g_s^*}^T {G_s^*}^{-1}(\boldsymbol{y}_{(t-s+1):t} - \mathbf{0}_m) \\
&= {g_s^*}^T {G_s^*}^{-1}\boldsymbol{y}_{(t-s+1):t} \\
&= {\Phi_s^*}^T \boldsymbol{y}_{(t-s+1):t}
\end{aligned}$$

for $s = 1, \ldots, p$, by definition. Therefore

$$\Phi_s^* = {G_s^*}^{-1} g_s^* \iff g_s^* = G_s^* \Phi_s^*, \quad s = 1, \ldots, p, \tag{S3}$$

in which we refer to the equations on the right as the *reverse prediction equations.*

The corresponding conditional variance is given by

$$\begin{aligned}
\operatorname{Var}(\boldsymbol{y}_{t-s}|\boldsymbol{y}_{(t-s+1):t}) &= \operatorname{Var}(\boldsymbol{y}_{t-s}) + \operatorname{Cov}(\boldsymbol{y}_{t-s}, \boldsymbol{y}_{(t-s+1):t})\operatorname{Var}(\boldsymbol{y}_{(t-s+1):t})^{-1}\operatorname{Cov}(\boldsymbol{y}_{(t-s+1):t}, \boldsymbol{y}_{t-s}) \\
&= \Gamma_0 - {g_s^*}^T {G_s^*}^{-1} g_s^* \\
&= \Gamma_0 - {g_s^*}^T \Phi_s^* \\
&= \Sigma_s^*
\end{aligned}$$

for $s = 1, \ldots, p$, by definition. By symmetry, this gives

$$\Sigma_s^* = \Gamma_0 - {\Phi_s^*}^T g_s^*, \quad s = 1, \ldots, p. \tag{S4}$$

Before proceeding with the proofs of the forward and reverse mapping, we use the properties of $Q$ and the forward and reverse prediction equations to derive the following preliminary results

$$Q\Phi_s = QG_s^{-1} g_s = (QG_sQ)^{-1} Qg_s = {G_s^*}^{-1} \tilde{g}_s \tag{S5}$$

for $s = 1, \ldots, p$. Similarly,

$$Q\Phi_s^* = Q{G_s^*}^{-1} g_s^* = (QG_s^*Q)^{-1} Qg_s^* = G_s^{-1} \tilde{g}_s^* \tag{S6}$$

for $s = 1, \ldots, p$.

## S2.2 Forward mapping

Now, for $s = 1$, the forward prediction equation simplifies to give

$$g_1 = G_1 \mathit{\Phi}_1 \iff \mathit{\Gamma}_1 = \mathit{\Gamma}_0 \phi_{11}^T$$

and so

$$\phi_{11} = \mathit{\Gamma}_1^T \mathit{\Gamma}_0^{-1} = \mathit{\Gamma}_1^T \mathit{\Sigma}_0^{*\,-1}. \tag{S7}$$

Similarly, from the first reverse prediction equation, we arrive at

$$g_1^* = G_1^* \mathit{\Phi}_1^* \iff \mathit{\Gamma}_1^T = \mathit{\Gamma}_0 \phi_{11}^{*\,T}$$

and so

$$\phi_{11}^* = \mathit{\Gamma}_1 \mathit{\Gamma}_0^{-1} = \mathit{\Gamma}_1 \mathit{\Sigma}_0^{-1}. \tag{S8}$$

For $s = 2, \ldots, p$ we can partition the matrices in the forward prediction equation, $G_s \mathit{\Phi}_s = g_s$, as follows

$$\begin{pmatrix} G_{s-1} & \tilde{g}_{s-1}^* \\ \tilde{g}_{s-1}^{*\,T} & \mathit{\Gamma}_0 \end{pmatrix} \begin{pmatrix} \mathit{\Phi}_{s,-s} \\ \phi_{ss}^T \end{pmatrix} = \begin{pmatrix} g_{s-1} \\ \mathit{\Gamma}_s \end{pmatrix}$$

or, equivalently,

$$G_{s-1} \mathit{\Phi}_{s,-s} + \tilde{g}_{s-1}^* \phi_{ss}^T = g_{s-1}, \tag{S9}$$
$$\tilde{g}_{s-1}^{*\,T} \mathit{\Phi}_{s,-s} + \mathit{\Gamma}_0 \phi_{ss}^T = \mathit{\Gamma}_s. \tag{S10}$$

Similarly, for $s = 2, \ldots, p$ we can partition the matrices in the backward prediction equation, $G_s^* \mathit{\Phi}_s^* = g_s^*$, as follows

$$\begin{pmatrix} G_{s-1}^* & \tilde{g}_{s-1} \\ \tilde{g}_{s-1}^T & \mathit{\Gamma}_0 \end{pmatrix} \begin{pmatrix} \mathit{\Phi}_{s,-s}^* \\ \phi_{ss}^{*\,T} \end{pmatrix} = \begin{pmatrix} g_{s-1}^* \\ \mathit{\Gamma}_s^T \end{pmatrix}$$

or, equivalently,

$$G_{s-1}^* \mathit{\Phi}_{s,-s}^* + \tilde{g}_{s-1} \phi_{ss}^{*\,T} = g_{s-1}^*, \tag{S11}$$
$$\tilde{g}_{s-1}^T \mathit{\Phi}_{s,-s}^* + \mathit{\Gamma}_0 \phi_{ss}^{*\,T} = \mathit{\Gamma}_s^T. \tag{S12}$$

From (S9) we can write

$$\mathit{\Phi}_{s,-s} = G_{s-1}^{-1}(g_{s-1} - \tilde{g}_{s-1}^* \phi_{ss}^T) = G_{s-1}^{-1} g_{s-1} - G_{s-1}^{-1} \tilde{g}_{s-1}^* \phi_{ss}^T$$

and then using (S1) and (S6) we have

$$\mathit{\Phi}_{s,-s} = \mathit{\Phi}_{s-1} - Q \mathit{\Phi}_{s-1}^* \phi_{ss}^T. \tag{S13}$$

So, blockwise, we have

$$\phi_{s,i} = \phi_{s-1,i} - \phi_{ss} \phi_{s-1,s-i}^*, \quad s = 2, \ldots, p,\ i = 1, \ldots, s-1. \tag{S14}$$

Similarly, from (S11) we can write

$$\mathit{\Phi}_{s,-s}^* = G_{s-1}^{*\,-1}(g_{s-1}^* - \tilde{g}_{s-1} \phi_{ss}^{*\,T}) = G_{s-1}^{*\,-1} g_{s-1}^* - G_{s-1}^{*\,-1} \tilde{g}_{s-1} \phi_{ss}^{*\,T}$$

and then using (S3) and (S5) we have

$$\mathit{\Phi}_{s,-s}^* = \mathit{\Phi}_{s-1}^* - Q \mathit{\Phi}_{s-1} \phi_{ss}^{*\,T}. \tag{S15}$$

So, blockwise, we have

$$\phi^*_{s,i} = \phi^*_{s-1,i} - \phi^*_{ss}\phi_{s-1,s-i}, \quad s = 2, \dots, p,\ i = 1, \dots, s-1. \tag{S16}$$

Equations (S14) and (S16) establish the results of (17) in the forward mapping from Appendix A.1 of the paper.

Next, taking (S13) in (S10) and using properties of $Q$ we can write

$$\begin{aligned}
\mathit{\Gamma}_0\phi^T_{ss} &= \mathit{\Gamma}_s - \tilde{g}^{*T}_{s-1}\mathit{\Phi}_{s,-s} \\
&= \mathit{\Gamma}_s - \tilde{g}^{*T}_{s-1}(\mathit{\Phi}_{s-1} - Q\mathit{\Phi}^*_{s-1}\phi^T_{ss}) \\
&= \mathit{\Gamma}_s - \tilde{g}^{*T}_{s-1}\mathit{\Phi}_{s-1} + (Qg^*_{s-1})^T Q\mathit{\Phi}^*_{s-1}\phi^T_{ss} \\
&= \mathit{\Gamma}_s - \tilde{g}^{*T}_{s-1}\mathit{\Phi}_{s-1} + g^{*T}_{s-1}\mathit{\Phi}^*_{s-1}\phi^T_{ss}.
\end{aligned}$$

We therefore have

$$\phi_{ss}(\mathit{\Gamma}_0 - \mathit{\Phi}^{*T}_{s-1}g^*_{s-1}) = \mathit{\Gamma}^T_s - \mathit{\Phi}^T_{s-1}\tilde{g}^*_{s-1}$$

which, from (S4), is equal to

$$\phi_{ss}\mathit{\Sigma}^*_{s-1} = \mathit{\Gamma}^T_s - \mathit{\Phi}^T_{s-1}\tilde{g}^*_{s-1}. \tag{S17}$$

Solving for $\phi_{ss}$, we can write

$$\phi_{ss} = (\mathit{\Gamma}^T_s - \mathit{\Phi}^T_{s-1}\tilde{g}^*_{s-1})\mathit{\Sigma}^{*-1}_{s-1} = (\mathit{\Gamma}^T_s - \phi_{s-1,1}\mathit{\Gamma}^T_{s-1} - \dots - \phi_{s-1,s-1}\mathit{\Gamma}^T_1)\mathit{\Sigma}^{*-1}_{s-1}, \quad s = 1, \dots, p. \tag{S18}$$

which encompasses (S7) as a special case in which $\mathit{\Phi}^T_0\tilde{g}^*_0 \equiv 0_m$.

Similarly, taking (S15) in (S12) and using properties of $Q$ we can write

$$\begin{aligned}
\mathit{\Gamma}_0\phi^{*T}_{ss} &= \mathit{\Gamma}^T_s - \tilde{g}^T_{s-1}\mathit{\Phi}^*_{s,-s} \\
&= \mathit{\Gamma}^T_s - \tilde{g}^T_{s-1}(\mathit{\Phi}^*_{s-1} - Q\mathit{\Phi}_{s-1}\phi^{*T}_{ss}) \\
&= \mathit{\Gamma}^T_s - \tilde{g}^T_{s-1}\mathit{\Phi}^*_{s-1} + (Qg_{s-1})^T Q\mathit{\Phi}_{s-1}\phi^{*T}_{ss} \\
&= \mathit{\Gamma}^T_s - \tilde{g}^T_{s-1}\mathit{\Phi}^*_{s-1} + g^T_{s-1}\mathit{\Phi}_{s-1}\phi^{*T}_{ss}.
\end{aligned}$$

We therefore have

$$\phi^*_{ss}(\mathit{\Gamma}_0 - \mathit{\Phi}^T_{s-1}g_{s-1}) = \mathit{\Gamma}_s - \mathit{\Phi}^{*T}_{s-1}\tilde{g}_{s-1}$$

which, from (S2) is equal to

$$\phi^*_{ss}\mathit{\Sigma}_{s-1} = \mathit{\Gamma}_s - \mathit{\Phi}^{*T}_{s-1}\tilde{g}_{s-1}. \tag{S19}$$

Solving for $\phi^*_{ss}$, we can write

$$\phi^*_{ss} = (\mathit{\Gamma}_s - \mathit{\Phi}^{*T}_{s-1}\tilde{g}_{s-1})\mathit{\Sigma}^{-1}_{s-1} = (\mathit{\Gamma}_s - \phi^*_{s-1,1}\mathit{\Gamma}_{s-1} - \dots - \phi^*_{s-1,s-1}\mathit{\Gamma}_1)\mathit{\Sigma}^{-1}_{s-1}, \quad s = 1, \dots, p \tag{S20}$$

which encompasses (S8) as a special case in which $\mathit{\Phi}^{*T}_0\tilde{g}_0 \equiv 0_m$. Equations (S18) and (S20) establish the results in (16) of the forward mapping.

The recursion for the matrices of autoregressive coefficients in the $s$-th forward and reverse prediction equations involve the conditional variances $\mathit{\Sigma}_{s-1}$ and $\mathit{\Sigma}^*_{s-1}$ for $s = 1, \dots, p-1$ and so we need to define a recursion for their computation.

Post-multiplying either side of (1) by $\boldsymbol{y}^T_{t+1}$ and taking expectations yields

$$\mathrm{E}(\boldsymbol{y}_{t+1}\boldsymbol{y}^T_{t+1}) = \sum_{i=1}^{s}\phi_{si}\mathrm{E}(\boldsymbol{y}_{t-i+1}\boldsymbol{y}^T_{t+1}) + \mathrm{E}(\boldsymbol{\epsilon}_{s,t+1}\boldsymbol{y}^T_{t+1}) \iff \mathit{\Gamma}_0 = \sum_{i=1}^{s}\phi_{si}\mathit{\Gamma}_i + \mathit{\Sigma}_s$$

and so

$$\Sigma_s = \Gamma_0 - \phi_{s1}\Gamma_1 - \ldots \phi_{ss}\Gamma_s, \quad s = 1, \ldots, p. \tag{S21}$$

Similarly, post-multiplying either side of (2) by $\boldsymbol{y}_{t-s}^T$ and taking expectations yields

$$\mathrm{E}(\boldsymbol{y}_{t-s}\boldsymbol{y}_{t-s}^T) = \sum_{i=1}^{s} \phi_{si}^* \mathrm{E}(\boldsymbol{y}_{t-s+i}\boldsymbol{y}_{t-s}^T) + \mathrm{E}(\boldsymbol{\epsilon}_{s,t-s}^* \boldsymbol{y}_{t-s}^T) \quad \Longleftrightarrow \quad \Gamma_0 = \sum_{i=1}^{s} \phi_{si}^* \Gamma_i^T + \Sigma_s^*$$

and so

$$\Sigma_s^* = \Gamma_0 - \phi_{s1}^*\Gamma_1^T - \ldots \phi_{ss}^*\Gamma_s^T, \quad s = 1, \ldots, p. \tag{S22}$$

Equations (S21) and (S22) establish the results of (19) in the forward mapping.

Recall that we define the partial autocorrelation matrices $P_1, \ldots, P_p$ as $P_{s+1} = \mathrm{Cov}(\boldsymbol{z}_{s,t+1}, \boldsymbol{z}_{s,t-s}^*)$ for $s = 0, \ldots, p-1$. For $s = 0$, we can write this as

$$P_1 = \mathrm{Cov}(S_0^{-1}\boldsymbol{y}_{t+1}\,,\, S_0^{*\,-1}\boldsymbol{y}_t) = S_0^{-1}\mathrm{Cov}(\boldsymbol{y}_{t+1}, \boldsymbol{y}_t)(S_0^{*\,T})^{-1} = S_0^{-1}\Gamma_1^T(S_0^{*\,T})^{-1}$$

which, using (S7), can be expressed as

$$P_1 = S_0^{-1}\phi_{11}\Sigma_0^*(S_0^{*\,T})^{-1} = S_0^{-1}\phi_{11}S_0^*S_0^{*\,T}(S_0^{*\,T})^{-1} = S_0^{-1}\phi_{11}S_0^*. \tag{S23}$$

Now, for $s = 1, \ldots, p-1$ we have

$$P_{s+1} = \mathrm{Cov}(S_s^{-1}\boldsymbol{\epsilon}_{s,t+1}\,,\, S_s^{*\,-1}\boldsymbol{\epsilon}_{s,t-s}^*) = S_s^{-1}\mathrm{Cov}(\boldsymbol{\epsilon}_{s,t+1}, \boldsymbol{\epsilon}_{s,t-s}^*)(S_s^{*\,T})^{-1}.$$

We can write the inner covariance as

$$\begin{aligned}
\mathrm{Cov}(\boldsymbol{\epsilon}_{s,t+1}, \boldsymbol{\epsilon}_{s,t-s}^*) &= \mathrm{Cov}(\boldsymbol{y}_{t+1} - \Phi_s^T\boldsymbol{y}_{t:t-s+1}\,,\, \boldsymbol{y}_{t-s} - \Phi_s^{*\,T}\boldsymbol{y}_{t-s+1:t}) \\
&= \mathrm{Cov}(\boldsymbol{y}_{t+1}, \boldsymbol{y}_{t-s}) - \mathrm{Cov}(\boldsymbol{y}_{t+1}, \boldsymbol{y}_{t-s+1:t})\Phi_s^* - \Phi_s^T\mathrm{Cov}(\boldsymbol{y}_{t:t-s+1}, \boldsymbol{y}_{t-s}) \\
&\qquad + \Phi_s^T\mathrm{Cov}(\boldsymbol{y}_{t:t-s+1}, \boldsymbol{y}_{t-s+1:t})\Phi_s^* \\
&= \mathrm{Cov}(\boldsymbol{y}_{t+1}, \boldsymbol{y}_{t-s}) - \mathrm{Cov}(\boldsymbol{y}_{t+1}, Q\boldsymbol{y}_{t:t-s+1})\Phi_s^* - \Phi_s^T\mathrm{Cov}(\boldsymbol{y}_{t:t-s+1}, \boldsymbol{y}_{t-s}) \\
&\qquad + \Phi_s^T\mathrm{Cov}(\boldsymbol{y}_{t:t-s+1}, Q\boldsymbol{y}_{t:t-s+1})\Phi_s^* \\
&= \Gamma_{s+1}^T - g_s^TQ\Phi_s^* - \Phi_s^T\tilde{g}_s^* + \Phi_s^TG_sQ\Phi_s^*.
\end{aligned}$$

Using (S6), this can be written as

$$\mathrm{Cov}(\boldsymbol{\epsilon}_{s,t+1}, \boldsymbol{\epsilon}_{s,t-s}^*) = \Gamma_{s+1}^T - g_s^TG_s^{-1}\tilde{g}_s^* - \Phi_s^T\tilde{g}_s^* + \Phi_s^TG_sG_s^{-1}\tilde{g}_s^*$$

which, using (S1), gives

$$\mathrm{Cov}(\boldsymbol{\epsilon}_{s,t+1}, \boldsymbol{\epsilon}_{s,t-s}^*) = \Gamma_{s+1}^T - \Phi_s^T\tilde{g}_s^*.$$

Finally, from (S17) we obtain

$$\mathrm{Cov}(\boldsymbol{\epsilon}_{s,t+1}, \boldsymbol{\epsilon}_{s,t-s}^*) = \phi_{s+1,s+1}\Sigma_s^*.$$

It follows that

$$P_{s+1} = S_s^{-1}\phi_{s+1,s+1}\Sigma_s^*(S_s^{*\,T})^{-1} = S_s^{-1}\phi_{s+1,s+1}S_s^*S_s^{*\,T}(S_s^{*\,T})^{-1}.$$

Therefore, also taking account of (S23), we have

$$P_{s+1} = S_s^{-1}\phi_{s+1,s+1}S_s^*, \quad s = 0, \ldots, p-1. \tag{S24}$$

To obtain an alternative representation of the partial autocorrelation matrices, it is instructive to construct $P_{s+1}^T$ for $s = 0, \dots, p-1$. For $s = 0$ we can write

$$P_1^T = \mathrm{Cov}(S_0^{*\,-1}\boldsymbol{y}_t\,,\, S_0^{-1}\boldsymbol{y}_{t+1}) = S_0^{*\,-1}\mathrm{Cov}(\boldsymbol{y}_t, \boldsymbol{y}_{t+1})(S_0^T)^{-1} = S_0^{*\,-1}\mathit{\Gamma}_1(S_0^T)^{-1}$$

which, using (S8), can be expressed as

$$P_1^T = S_0^{*\,-1}\phi_{11}^*\mathit{\Sigma}_0(S_0^T)^{-1} = S_0^{*\,-1}\phi_{11}^* S_0 S_0^T(S_0^T)^{-1} = S_0^{*\,-1}\phi_{11}^* S_0$$

and so

$$P_1 = (S_0^{*\,-1}\phi_{11}^* S_0)^T. \tag{S25}$$

Now, for $s = 1, \dots, p-1$ we can write

$$P_{s+1}^T = \mathrm{Cov}(S_s^{*\,-1}\boldsymbol{\epsilon}_{s,t-s}^*\,,\, S_s^{-1}\boldsymbol{\epsilon}_{s,t+1}) = S_s^{*\,-1}\mathrm{Cov}(\boldsymbol{\epsilon}_{s,t-s}^*, \boldsymbol{\epsilon}_{s,t+1})(S_s^T)^{-1}.$$

The inner covariance can be expressed as

$$\begin{aligned}
\mathrm{Cov}(\boldsymbol{\epsilon}_{s,t-s}^*, \boldsymbol{\epsilon}_{s,t+1}) &= \mathrm{Cov}(\boldsymbol{y}_{t-s} - \mathit{\Phi}_s^{*\,T}\boldsymbol{y}_{t-s+1:t}\,,\, \boldsymbol{y}_{t+1} - \mathit{\Phi}_s^T\boldsymbol{y}_{t:t-s+1})\\
&= \mathrm{Cov}(\boldsymbol{y}_{t-s}, \boldsymbol{y}_{t+1}) - \mathrm{Cov}(\boldsymbol{y}_{t-s}, \boldsymbol{y}_{t:t-s+1})\mathit{\Phi}_s - \mathit{\Phi}_s^{*\,T}\mathrm{Cov}(\boldsymbol{y}_{t-s+1:t}, \boldsymbol{y}_{t+1})\\
&\qquad + \mathit{\Phi}_s^{*\,T}\mathrm{Cov}(\boldsymbol{y}_{t-s+1:t}, \boldsymbol{y}_{t:t-s+1})\mathit{\Phi}_s\\
&= \mathrm{Cov}(\boldsymbol{y}_{t-s}, \boldsymbol{y}_{t+1}) - \mathrm{Cov}(\boldsymbol{y}_{t-s}, Q\boldsymbol{y}_{t-s+1:t})\mathit{\Phi}_s - \mathit{\Phi}_s^{*\,T}\mathrm{Cov}(\boldsymbol{y}_{t-s+1:t}, \boldsymbol{y}_{t+1})\\
&\qquad + \mathit{\Phi}_s^{*\,T}\mathrm{Cov}(\boldsymbol{y}_{t-s+1:t}, Q\boldsymbol{y}_{t-s+1:t})\mathit{\Phi}_s\\
&= \mathit{\Gamma}_{s+1} - g_s^{*\,T}Q\mathit{\Phi}_s - \mathit{\Phi}_s^{*\,T}\tilde{g}_s + \mathit{\Phi}_s^{*\,T}G_s^*Q\mathit{\Phi}_s.
\end{aligned}$$

Using (S5), this can be written as

$$\mathrm{Cov}(\boldsymbol{\epsilon}_{s,t-s}^*, \boldsymbol{\epsilon}_{s,t+1}) = \mathit{\Gamma}_{s+1} - g_s^{*\,T}G_s^{*\,-1}\tilde{g}_s - \mathit{\Phi}_s^{*\,T}\tilde{g}_s + \mathit{\Phi}_s^{*\,T}G_s^*G_s^{*\,-1}\tilde{g}_s$$

which, using (S3), gives

$$\mathrm{Cov}(\boldsymbol{\epsilon}_{s,t-s}^*, \boldsymbol{\epsilon}_{s,t+1}) = \mathit{\Gamma}_{s+1} - \mathit{\Phi}_s^{*\,T}\tilde{g}_s.$$

Finally, from (S19) we obtain

$$\mathrm{Cov}(\boldsymbol{\epsilon}_{s,t-s}^*, \boldsymbol{\epsilon}_{s,t+1}) = \phi_{s+1,s+1}^*\mathit{\Sigma}_s.$$

It follows that

$$P_{s+1}^T = S_s^{*\,-1}\phi_{s+1,s+1}^*\mathit{\Sigma}_s(S_s^T)^{-1} = S_s^{*\,-1}\phi_{s+1,s+1}^* S_s S_s^T(S_s^T)^{-1} = S_s^{*\,-1}\phi_{s+1,s+1}^* S_s.$$

Therefore, also taking account of (S25), we can write the partial autocorrelation matrices as

$$P_{s+1} = (S_s^{*\,-1}\phi_{s+1,s+1}^* S_s)^T, \quad s = 0, \dots, p-1. \tag{S26}$$

Equations (S24) and (S26) establish the results of (18) in the forward mapping.

It is also clear that

$$\mathrm{Cov}(\boldsymbol{y}_{t+1}, \boldsymbol{y}_t) = \mathrm{Cov}(\boldsymbol{y}_t, \boldsymbol{y}_{t+1})^T \quad \Longleftrightarrow \quad \phi_{11}\mathit{\Sigma}_0^* = (\phi_{11}^*\mathit{\Sigma}_0)^T$$

and, for $s = 1, \dots, p-1$, that

$$\mathrm{Cov}(\boldsymbol{\epsilon}_{s,t+1}, \boldsymbol{\epsilon}_{s,t-s}^*) = \mathrm{Cov}(\boldsymbol{\epsilon}_{s,t-s}^*, \boldsymbol{\epsilon}_{s,t+1})^T \quad \Longleftrightarrow \quad \phi_{s+1,s+1}\mathit{\Sigma}_s^* = (\phi_{s+1,s+1}^*\mathit{\Sigma}_s)^T.$$

Therefore we have

$$\phi_{s+1,s+1}\mathit{\Sigma}_s^* = (\phi_{s+1,s+1}^*\mathit{\Sigma}_s)^T, \quad s = 0, \dots, p-1 \tag{S27}$$

### S2.3 Reverse mapping

In the reverse mapping, the results in (21) from Appendix A.2 of the paper follow from trivial rearrangement of the results in (18) in the forward mapping from Appendix A.1. The equations (22) are unchanged from (17) and equation (24) follows from direct rearrangement of the first equation in (16).

For $s = 0, \ldots, p-1$ we can partition the matrices in the expression for the conditional variance, $\Sigma_{s+1} = \Gamma_0 - \Phi_{s+1}^T g_{s+1}$, as follows

$$\begin{aligned}\Sigma_{s+1} &= \Gamma_0 - \begin{pmatrix}\Phi_{s+1,-(s+1)}^T & \phi_{s+1,s+1}\end{pmatrix}\begin{pmatrix}g_s \\ \Gamma_{s+1}\end{pmatrix} \\ &= \Gamma_0 - \Phi_{s+1,-(s+1)}^T g_s - \phi_{s+1,s+1}\Gamma_{s+1}\end{aligned}$$

which, using (S13), yields

$$\begin{aligned}\Sigma_{s+1} &= \Gamma_0 - (\Phi_s^T - \phi_{s+1,s+1}\Phi_s^{*\,T} Q)g_s - \phi_{s+1,s+1}\Gamma_{s+1} \\ &= \Gamma_0 - \Phi_s^T g_s - \phi_{s+1,s+1}(\Gamma_{s+1} - \Phi_s^{*\,T}\tilde{g}_s)\end{aligned}$$

and then using (S2) and (S19) gives

$$\Sigma_{s+1} = \Sigma_s - \phi_{s+1,s+1}\phi_{s+1,s+1}^*\Sigma_s. \tag{S28}$$

Finally, from (S27) we have

$$\Sigma_{s+1} = \Sigma_s - \phi_{s+1,s+1}\Sigma_s^*\phi_{s+1,s+1}^T, \quad s = 0, \ldots, p-1. \tag{S29}$$

For $s = 0, \ldots, p-1$ we can partition the matrices in the expression for the conditional variance, $\Sigma_{s+1}^* = \Gamma_0 - \Phi_{s+1}^{*\,T} g_{s+1}^*$, as follows

$$\begin{aligned}\Sigma_{s+1}^* &= \Gamma_0 - \begin{pmatrix}\Phi_{s+1,-(s+1)}^{*\,T} & \phi_{s+1,s+1}^*\end{pmatrix}\begin{pmatrix}g_s^* \\ \Gamma_{s+1}^T\end{pmatrix} \\ &= \Gamma_0 - \Phi_{s+1,-(s+1)}^{*\,T} g_s^* - \phi_{s+1,s+1}^*\Gamma_{s+1}^T\end{aligned}$$

which, using (S15), yields

$$\begin{aligned}\Sigma_{s+1}^* &= \Gamma_0 - (\Phi_s^{*\,T} - \phi_{s+1,s+1}^*\Phi_s^T Q)g_s^* - \phi_{s+1,s+1}^*\Gamma_{s+1}^T \\ &= \Gamma_0 - \Phi_s^{*\,T} g_s^* - \phi_{s+1,s+1}^*(\Gamma_{s+1}^T - \Phi_s^T\tilde{g}_s^*)\end{aligned}$$

and then using (S4) and (S17) gives

$$\Sigma_{s+1}^* = \Sigma_s^* - \phi_{s+1,s+1}^*\phi_{s+1,s+1}\Sigma_s^*.$$

Finally, from (S27) we have

$$\Sigma_{s+1}^* = \Sigma_s^* - \phi_{s+1,s+1}^*\Sigma_s\phi_{s+1,s+1}^{*\,T}, \quad s = 0, \ldots, p-1. \tag{S30}$$

Equations (S29) and (S30) establish the results of (23) in the reverse mapping.

Finally, using (21) we can write (S28) as

$$\begin{aligned}\Sigma_{s+1} &= \Sigma_s - \phi_{s+1,s+1}\phi_{s+1,s+1}^*\Sigma_s \\ &= S_s S_s^T - (S_s P_{s+1} S_s^{*\,-1})(S_s^* P_{s+1}^T S_s^{-1}) S_s S_s^T \\ &= S_s S_s^T - S_s P_{s+1} P_{s+1}^T S_s^T \\ &= S_s(I_m - P_{s+1}P_{s+1}^T)S_s^T, \quad s = 0, \ldots, p-1, \end{aligned} \tag{S31}$$

Table S1: The variables in the macroeconomic time series and the models ($m$) in which they were used.

| Variable | $m$ |
|---|---|
| Real GDP: quantity index (2000 = 100) | $3, 10, 20$ |
| CPI: all items | $3, 10, 20$ |
| Interest rate: federal funds (e_ective) (percentage per annum) | $3, 10, 20$ |
| Real spot market price index: all commodities | $10, 20$ |
| Depository institution reserves: nonborrowed (millions of dollars) | $10, 20$ |
| Depository institution reserves: total (millions of dollars) | $10, 20$ |
| Money stock: M2 (billions of dollars) | $10, 20$ |
| Real Personal Consumption Expenditures: quantity index | $10, 20$ |
| Industrial production index: total | $10, 20$ |
| Capacity utilization: manufacturing (SIC) | $10, 20$ |
| Unemployment rate: all workers, 16 and over (percentage) | 20 |
| Housing starts: total (thousands) | 20 |
| Producer price index: finished goods | 20 |
| Personal Consumption Expenditures: price index | 20 |
| Real average hourly earnings: non-farm production workers | 20 |
| Money stock: M1 (billions of dollars) | 20 |
| S&P's common stock price index: industrials | 20 |
| Interest rate: US treasury constant maturity, 10-year | 20 |
| US effective exchange rate: index number | 20 |
| Employees, non-farm: total private | 20 |

in which $I_m - P_{s+1}P_{s+1}^T$ is positive semi-definite (Ansley and Kohn, 1986). Equation (S31) establishes (20) from the reverse mapping.

If $S_s$ is the lower triangular Cholesky factor of $\mathit{\Sigma}_s$, then we decompose $(I_m - P_{s+1}P_{s+1}^T)$ according to its Cholesky decomposition which we write as

$$I_m - P_{s+1}P_{s+1}^T = B_{s+1}^{-1}B_{s+1}^{-1\,T},$$

where $B_{s+1}^{-1}$ is lower triangular, and then solve (S31) for $S_s$ through

$$S_s = S_{s+1}B_{s+1}.$$

If $S_s$ is the symmetric matrix-square-root of $\mathit{\Sigma}_s$, then we denote by $B_{s+1}^{-1}$ the symmetric matrix-square-root of $(I_m - P_{s+1}P_{s+1}^T)$ and then solve (S31) for $S_s$ through

$$S_s = B_{s+1}(B_{s+1}^{-1}\mathit{\Sigma}_{s+1}B_{s+1}^{-1})^{1/2}B_{s+1}.$$

# S3 Application

Table S1 indicates which variables in the macroeconomic time series analysed in the manuscript were used in the $\text{VAR}_3(4)$, $\text{VAR}_{10}(4)$ and $\text{VAR}_{20}(4)$ models.

In the Minnesota and semi-conjugate priors used in the application, every element of $\mathit{\Phi}$ was taken to be independent, so that the prior variance matrices $W_{2,s}$ and $W_{3,s}$ were diagonal. The prior means in $\boldsymbol{m}_{2,s}$ and $\boldsymbol{m}_{3,s}$, $s = 1, \dots, p$, were chosen to be zero in all analyses. Within each matrix $\phi_s$, the diagonal elements were all assigned the same variance and similarly for the off-diagonal elements. The specification is indicated in Table S2. These choices were made to approximately match the marginal prior means and variances for $\mathit{\Phi}$ induced by our exchangeable stationary prior.

Table S2: The standard deviations for the diagonal and off-diagonal elements in $\phi_1, \ldots, \phi_4$ in the Minnesota and semi-conjugate prior for each value of $m$.

| $m$ | Diagonal | | | | Off-diagonal | | | |
|---|---|---|---|---|---|---|---|---|
| | $\phi_1$ | $\phi_2$ | $\phi_3$ | $\phi_4$ | $\phi_1$ | $\phi_2$ | $\phi_3$ | $\phi_4$ |
| 3 | 1.4 | 1.7 | 1.4 | 0.7 | 1.7 | 2.0 | 1.7 | 0.9 |
| 10 | 6.0 | 8.6 | 6.5 | 1.0 | 6.0 | 8.8 | 6.7 | 1.0 |
| 20 | 15.0 | 22.0 | 15.5 | 1.2 | 15.0 | 22.0 | 15.5 | 1.2 |

# References

Ansley, C. F. and R. Kohn (1986). A note on reparameterizing a vector autoregressive moving average model to enforce stationarity. *Journal of Statistical Computation and Simulation 24*, 99–106.
